# Supplementary material for: Driftfusion: An open source code for simulating ordered semiconductor devices with mixed ionic-electronic conducting materials in one-dimension
Source: arXiv:2009.04384 source file (2022-01-05)
Supplement: Supplementary file 1 [file LstS2_build_device_SI.tex]

function dev = build_device(par, meshoption)
% BUILD_DEVICE calls BUILD_PROPERTY for each device property. BUILD_PROPERTY then defines the
% properties at each point on the grid defined by MESHOPTION

switch meshoption
    case 'whole'
        xmesh = par.xx;
    case 'sub'
        xmesh = par.x_sub;
end

% Properties with constant values in the interfacial regions
% Constant properties
dev.mu_c = build_property(par.mu_c, xmesh, par, 'constant', 0);
dev.mu_a = build_property(par.mu_a, xmesh, par, 'constant', 0);
dev.epp = build_property(par.epp, xmesh, par, 'constant', 0);
dev.k_iongen = build_property(par.k_iongen, xmesh, par, 'constant', 0);
dev.k_ionrec = build_property(par.k_ionrec, xmesh, par, 'constant', 0);

% Linearly graded properties
dev.EA = build_property(par.EA, xmesh, par, 'lin_graded', 0);
dev.IP = build_property(par.IP, xmesh, par, 'lin_graded', 0);
dev.E0 = build_property(par.E0, xmesh, par, 'lin_graded', 0);

% Logarithmically graded properties
dev.NA = build_property(par.NA, xmesh, par, 'zeroed', 0);
dev.ND = build_property(par.ND, xmesh, par, 'zeroed', 0);
dev.Nc = build_property(par.Nc, xmesh, par, 'log_graded', 0);
dev.Nv = build_property(par.Nv, xmesh, par, 'log_graded', 0);
dev.n0 = build_property(par.n0, xmesh, par, 'log_graded', 0);
dev.p0 = build_property(par.p0, xmesh, par, 'log_graded', 0);
dev.Nani = build_property(par.Nani, xmesh, par, 'log_graded', 0);
dev.Ncat = build_property(par.Ncat, xmesh, par, 'log_graded', 0);
dev.ni = build_property(par.ni, xmesh, par, 'log_graded', 0);
dev.DOSani = build_property(par.amax, xmesh, par, 'log_graded', 0);
dev.DOScat = build_property(par.cmax, xmesh, par, 'log_graded', 0);

% Properties that are zeroed in the interfaces
dev.g0 = build_property(par.g0, xmesh, par, 'zeroed', 0);
dev.B = build_property(par.B, xmesh, par, 'zeroed', 0);

% Gradient properties
dev.gradEA = build_property(par.EA, xmesh, par, 'lin_graded', 1);
dev.gradIP = build_property(par.IP, xmesh, par, 'lin_graded', 1);
dev.gradNc = build_property(par.Nc, xmesh, par, 'log_graded', 1);
dev.gradNv = build_property(par.Nv, xmesh, par, 'log_graded', 1);

% Surface recombination velocity equivalence schemes
dev.mue = build_property(par.mue, xmesh, par, 'mue_interface', 0);
dev.muh = build_property(par.muh, xmesh, par, 'muh_interface', 0);
dev.taun = build_property(par.taun, xmesh, par, 'surface_rec_taun', 0);
dev.taup = build_property(par.taup, xmesh, par, 'surface_rec_taup', 0);
dev.nt = build_property(par.nt, xmesh, par, 'surface_rec_nt', 1);
dev.pt = build_property(par.pt, xmesh, par, 'surface_rec_pt', 1);
dev.ni_srh = build_property(par.ni, xmesh, par, 'surface_rec_ni_srh', 0);
dev.int_switch = build_property(par.int_switch, xmesh, par, 'int_switch', 0);

end
